# Supplementary material for: Identification of the surface features in the electronic structure of Cr
Source: arXiv:1506.07482 source file (2015-06-24)
Supplement: Supplementary file 1 [file Cr110_APL_suppl.pdf]

# Supplementary materials on 'Anomalies in the surface electronic structure of Cr'

Khadiza Ali, Shyama R. Varier, Deepnarayan Biswas, Srinivas C. Kandukuri, and Kalobaran Maiti[1]
*Department of Condensed Matter Physics and Materials Science, Tata Institute of Fundamental Research, Homi Bhabha Road, Colaba, Mumbai - 400 005, INDIA.*

( Dated: 20 June 2015)

Here we present the details of preparation and characterization of Cr(110) films on W(110) surface. Some details of the band structure calculations relevant for our studies are also presented. $X$-ray photoemission spectroscopic results are also presented exhibiting oxygen impurities on the surface emerged due to aging of the sample.

## I. SAMPLE PREPARATION AND CHARACTERIZATION

The Cr(110) surface was prepared in an ultrahigh vacuum chamber with a base pressure better than $1\times10^{-10}$ Torr and employing electron beam evaporation of Cr onto a clean W(110). Before the deposition of the Cr film, the W(110) surface was cleaned by heating it in oxygen pressure of $10^{-7}$ torr at 600 $^o$C for about a day with intermittent flashing at a temperature around 2500 $^o$C. The cleanliness of the sample surface was ensured by sharp low energy electron diffraction (LEED) pattern as shown in Fig. 1(a). In addition, we carried out $x$-ray photoemission spectroscopy (XPS) using a monochromatic Al $K\alpha$ source and Phoibos 150 analyzer from Specs to investigate trace of impurities in the material. The experimental technique is sufficiently bulk sensitive at this energy[1–3] and hence capable of revealing both surface and bulk impurities. The survey spectra shown in Fig. 1(b) exhibit absence of impurity feature in W(110) surface.

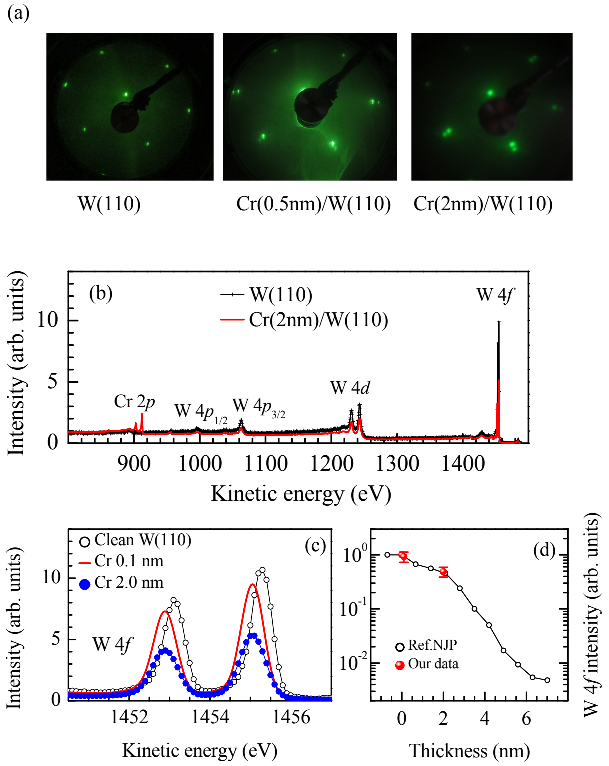


FIG. 1. Low energy electron diffraction (LEED) patterns of cleaned W(110) surface, Cr(0.5nm)/W(110) and Cr(2nm)/W(110) sample surfaces. (b) XPS survey spectrum of W(110) and Cr(2nm)/W(110) surfaces exhibiting absence of impurity and growth of Cr layers. (c) W $4f$ signal from differently covered W(110) surfaces exhibiting gradual decrease of W $4f$ intensity with increase in Cr overlayer thickness. (d) W $4f$ intensity is compared with previously published data from Ref. [1]

After ensuring the cleanliness and crystallinity of the substrate, we deposited Cr layer on the clean surface at a deposition rate of 2Å/min at room temperature. In order to achieve clean Cr film, the evaporator has been degassed for long time and characterized it to evaporate at $2\times10^{-10}$ torr vacuum. The as deposited films were annealed at about 600 $^o$C for 15 minutes. The crystallinity and the good quality of the surface was confirmed by sharp (1×1) LEED pattern. The evolution of the LEED pattern with the deposition of Cr layers is shown in Fig. 1(a). The middle LEED pattern in the figure exhibit emergence of the spots in addition of the LEED spots of W(110) surface at 0.5 nm coverage. The intensity of the Cr-related spots in the LEED patterns gradually increases with the increase in Cr layer thickness and become quite sharp at 2 nm thickness. Sharpness of the spots indicates good crystalline order of the film.

In order to investigate the presence of impurities in the films, we carried out XPS studies on the Cr(110) surface. The survey spectrum is superimposed on the W(110) spectrum in Fig. 1(b). We did not observe any signature of impurity feature indicating highly pure sample. The signature of Cr $2p$ signal in the kinetic energy range 900-920 eV emerges with Cr deposition and gradually increases with the increase in Cr film thickness along with a reduction in intensity of the W-related features.

The thickness of the Cr layer was determined by calibrating the evaporation rate using a quartz microbalance. The deposited Cr layer thickness was studied further by the intensity of W $4f$ signal as demonstrated in Fig. 1(c) and 1(d). The W $4f$ signal intensity gradually decreases with the increase in Cr-film thickness. We plot the W $4f$ intensity in Fig. 1(d) and demonstrate the consistency

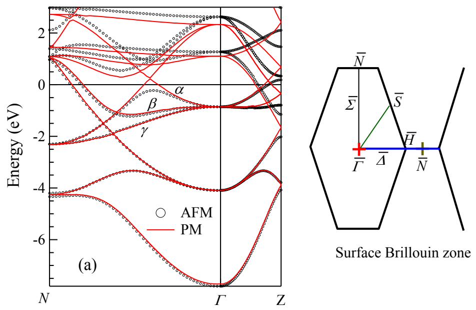


FIG. 2. (a) Calculated energy band structure along the $k$-vectors probed in the present experiments. Symbols and lines represent magnetically ordered and paramagnetic phase solution of the sample. The right panel shows the surface Brillouin zone and high symmetry points.

of our results with the published results[4].

## II. BAND STRUCTURE CALCULATION

The energy band structure of Cr has been calculated extensively in the past[5–7]. In order to investigate the energy bands along the $k$-vectors studied in this paper, we calculated the energy band structure considering the antiferromagnetic supercell employing full potential linearized augmented plane wave (FLAPW) method within the local spin density approximation (LSDA). Wien2k software has been used for the calculations[8]. We used 512 $k$-point to achieve the convergence.

The results for the antiferromagnetic (circles) and non-magnetic (lines) ground states are shown in Fig. 2(a). There are three energy bands denoted by $\alpha$, $\beta$ and $\gamma$ close to the Fermi level, $\epsilon_F$ and possess $t_{2g}$ symmetry. The degeneracy of these bands at $\Gamma$ is lifted at higher $k$-values in all the $k$-directions shown here. The $\alpha$ band makes an electron pocket around the $\Gamma$-point, the $\beta$ band makes a hole pocket around the high symmetry point, $N$ and the $\gamma$ bands disperses away from $\epsilon_F$ along $\Gamma N$. Along $\Gamma Z$, $\beta$ and $\gamma$ bands remain degenerate, while the $\alpha$ band crosses $\epsilon_F$.

Cr exhibits incommensurate SDW transition at 311 K with a periodicity close to 21 times the lattice constant. The Fermi surface nesting relevant to the emergence of SDW state involves the electron pocket around $\Gamma$ point[9,10]. Upon establishing the antiferromagnetic order, the $\alpha$-bands fold back opening up an energy gap of about 0.4 eV as demonstrated by the symbols in the figure. The other parts of the band structure remain quite similar in the occupied part for both magnetic and non-magnetic solutions.

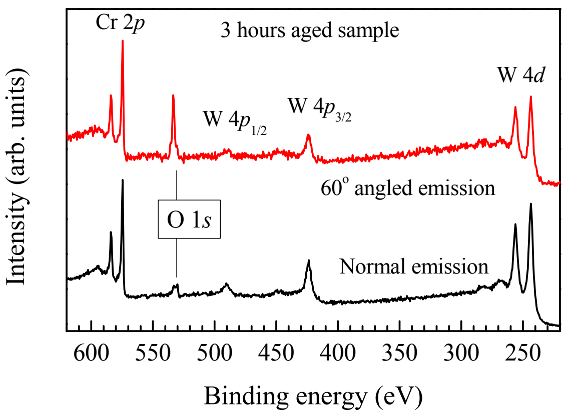


FIG. 3. $x$-ray photoemission spectra collected at 300 K from the 3 hours aged sample. The top panel correspond to $60^o$ angled emission and lower panel correspond to normal emission.

## III. X-RAY PHOTOEMISSION ON AGED SURFACE

We investigate the impurities due to aging in Fig. 3, where we show here the $x$-ray photoemission spectra collected with Al $K\alpha$ source at 300 K. The normal emission spectrum exhibit Cr $2p$, W $4d$ and W $4p$ signals. In addition, a weak feature around 530 eV binding energy is observed corresponding to O $1s$ emission, which was absent in the freshly prepared sample. The spectrum collected at $60^o$ emission angle exhibit significant enhancement of the O $1s$ signal intensity with subsequent decrease of W related signals. The increase in emission angle makes the technique more surface sensitive[1–3]. These results, thus, suggests that the oxygens are residing primarily on the sample surface.


[1] K. Maiti *et al.*, Phys. Rev. B **73**, 052508 (2006).
[2] R. S. Singh, V. R. R. Medicherla, K. Maiti and E. V. Sampathkumaran, Phys. Rev. B **77**, 201102 (2008).
[3] K. Maiti, R. S. Singh and V. R. R. Medicherla, Phys. Rev. B **76**, 165128 (2007).
[4] E. Rotenberg *et al.*, New J. Phys. **7,** 114 (2005).
[5] S. Asano and J. Yamashita, J. Phys. Soc. Jpn. **23**, 714 (1967).
[6] R. H. Victora and L. M. Falicov, Phys. Rev. B **31**, 7335 (1985).
[7] P. Habibi, C. Barreteau and A. Smogunov, J. Phys. Condens. Matter **25**, 146002 (2013).
[8] P. Blaha, K. Schwarz, G. K.H. Madsen, D. Kvasnicka and J. Luitz, **WIEN2k**, *An Augmented Plane Wave + Local Orbitals Program for Calculating Crystal Properties* (Karlheinz Schwarz, Techn. Universität Wien, Austria), 2001. ISBN 3-9501031-1-2.
[9] E. Fawcett, Rev. Mod. Phys. **60,** 209 (1988).
[10] J. Graebner and J. A. Marcus, J. Appl. Phys. **37**, 1262 (1966).
